# Supplementary material for: On the Concurrent Composition of Quantum Zero-Knowledge
Source: arXiv:2012.03139 source file (2021-07-18)
Supplement: Supplementary file 1 [file appendix.tex]

\section{General Cloning Security}
\label{sec:generalcloning}
The definition of reduction-friendly cloning security formulated earlier was closely tied to our security reduction. We could consider a more general and natural definition of cloning security, where we allow the QPT adversary to have access to a cloning oracle; that is, an oracle that on input a state $\ket{\Psi}$ and an integer $k$, outputs  $\ket{\Psi}^{\otimes k}$. We can furthermore parameterize this assumption with $q$, where $q$ is the number of queries made by the oracle. We note that QLWE is insecure against general cloning adversaries even if they make just one query; the attack is the same as the one presented in~\Cref{sec:rfc}.  
\par However, it is still  meaningful to investigate the security of other cryptographic concepts with respect to the general cloning security definition. For instance, does there exist a one-way function secure against general cloning adversaries? Answering this question in the affirmative  might open up the possibility of proving post-quantum security of existing interactive protocols. As an example, this might be useful in proving post-quantum security of interactive protocols that use hardcore bits~\cite{GL89}. In the security reduction, we  execute the adversary multiple times to break the one-way function and thus, in this scenario, cloning security might be useful. On the other hand, if the answer to the above question is no, then this might be useful in constructing primitives with uncloneability property; that is, primitives where cloning would violate the security definition (for example, quantum money). As an example,~\cite{RZ20} showed that SIS is insecure against general cloning adversaries and then turned this fact into a construction of franchised quantum money.
\par On the negative side, we show later, that any NP language can be solved by a general cloning algorithm making large number of queries. This rules out the existence of any cryptographic assumption secure against general cloning adverasries, where no upper bound is placed on the number of cloning queries made by the QPT adversary. 
\par We now formally introduce the notion of general cloning. 

\begin{definition}[$q$-General Cloning]
We say that a (non-uniform) QPT algorithm is a general cloning algorithm if it takes as input $x$ and makes $q$ queries to an oracle $\oracle$, where $\oracle$ is an oracle that takes as input $\ket{\Psi}$, integer $k$ and outputs $\ket{\Psi}^{\otimes k}$. 
\end{definition}

\par We investigate the power of general cloning algorithms. We show, in Section~\ref{subsec:adaptive}, that any NP language can be solved by a $q$-general cloning algorithm, for a large $q$. Moreover, even for $q=1$, it was shown in~\cite{RZ20} that SIS (and hence, LWE for the parameters we consider) is false even against 1-general cloning algorithms.

\subsection{Adaptive Attack}
\label{subsec:adaptive}
The following attack is based on a suggestion by Harrow~\cite{Aram2020}:  for any language $L$ in NP, there exists a quantum polynomial-time algorithm, making $q$ (adaptive) queries to the cloning oracle, that solves $L$. 

\begin{theorem}
Consider an NP relation $\rel=\{(x,w)\}$. Let the size of a witness associated with instance $x$ be upper bounded by $p(|x|)$. Then there exists a quantum polynomial-time algorithm, taking as input $x$, making $p(|x|)$ queries to oracle $\oracle$ (defined below), it outputs a witness $w$ for $x$ with probability $\geq \frac{1}{3}$. 
\par Oracle $\oracle$ takes as input a pure state and a positive integer, i.e. $(\ket{\Psi},k)$, and outputs $\ket{\Psi}^{\otimes k}$. 
\end{theorem}
\begin{proof}
Let $C$ be the verification circuit associated with $R$. We describe the algorithm in Figure~\ref{fig:adaptive_attack}.\\

\begin{figure}[!htb]
\begin{center}
\begin{tabular}{|p{15cm}|}
   \hline \\
   {\bf Input}: instance $x \in L$. Let $n$ be the size of the witness.\\
   \ \\
   \noindent Prepare the following state:
   \begin{eqnarray*}
   \ket{\Psi_0} & = & \sum_{y} \frac{1}{\sqrt{2^n}} \ket{y}\ket{C(x,y)} \\ 
   & = & \frac{1}{\sqrt{2^n}} \left( \sum_{y:C(x,y)=1} \ket{y} \ket{1} + \sum_{y:C(x,y) = 0} \ket{y}\ket{0} \right) \\
   & = & \sqrt{\varepsilon} \ket{\phi_1}\ket{1} + \sqrt{1-\varepsilon} \ket{\phi_0}\ket{0}
   \end{eqnarray*}
   For $i \in [n]$, do the following: 
   \begin{itemize}
        \item Let $\ket{\Psi_{i-1}}= \sqrt{\varepsilon_{i-1}}\ket{\phi_1}\ket{1} + \sqrt{\delta_{i-1}}\ket{\phi_0}\ket{0}$
        \item Query the oracle with $(\ket{\Psi_{i-1}},|x|)$ to obtain $\ket{\Psi_{i-1}}^{\otimes |x|}$. 
       \item For $j \in [|x|]$, do the following: 
       \begin{itemize}
           \item Measure $\ket{\Psi_{i-1}}$ with respect to $\{I \otimes M_0 , I \otimes M_1\}$, where: 
           $$M_0 = \frac{1}{\sqrt{2}} \ket{0}\bra{0} + \ket{1}\bra{1}$$
           $$M_1 = \frac{1}{\sqrt{2}} \ket{0}\bra{0}$$
         %  \item If the measurement outcome is 0 then the state obtained is 
         %  $$\ket{\Psi_i} =  \frac{(I \otimes M_0) \ket{\Psi_{i-1}}}{\sqrt{\alpha_{i-1}}} = \frac{1}{\sqrt{\alpha_{i-1}}} \left( \sqrt{\varepsilon_{i-1}} \ket{\phi_1}\ket{1} + \sqrt{\frac{\delta_{i-1}}{2}}\ket{\Psi_{i-1}}\ket{0} \right),$$
       %    where $\alpha_{i-1}=\bra{\Psi_{i-1}}M_0^{\dagger} M_0 \ket{\Psi_{i-1}}$.
         \item If the measurement outcome is 0, abort this loop and go to the $(i+1)^{th}$ execution. Let $\ket{\Psi_i}$ be the post-measurement state. Otherwise if the measurement outcome is 1, continue.
          
       \end{itemize}
   \item If in all the $|x|$ iterations, the measurement outcome is 1, output $\bot$.         
   \end{itemize}
   \ \\
   Measure the first register with respect to computational basis.\\ Output the resulting measurement outcome $y$.\\
   \ \\
      \hline
\end{tabular}
\end{center}
    \caption{Adaptive Attack}
    \label{fig:adaptive_attack}
\end{figure}
\ \\
\noindent  We now argue that with probability $\geq \frac{1}{3}$, the algorithm in Figure~\ref{fig:adaptive_attack} outputs a witness for $x$. 
\par We first argue how $\delta_i$ evolves during the computation by performing induction on $i$. The base case corresponds to $\delta_1$. Note that $\delta_1=\frac{\delta_0}{2\alpha_1}$, where $\delta_0=1-\varepsilon$. Moreover, $\alpha_1=\bra{\Psi_0}M_0^{\dagger}M_0 \ket{\Psi_0}=\frac{(1+\varepsilon)}{2}$. We now prove the induction hypothesis for $i \geq 2$. 

\begin{lemma}
Suppose $\delta_{i-1}=\frac{\delta_0}{\left( \prod_{j=1}^{i-1} \alpha_j \right) \cdot 2^{i-1}}$, where $\ket{\Psi_{i-1}}= \sqrt{\varepsilon_{i-1}}\ket{\phi_1}\ket{1} + \sqrt{\delta_{i-1}}\ket{\phi_0}\ket{0}$, is the state computed at the beginning of the $i^{th}$ iteration, where $\alpha_{j}=\bra{\Psi_{j-1}} M_0^{\dagger} M_0 \ket{\Psi_{j-1}} = \frac{(1 + (2^j - 1)\varepsilon)}{2^j}$.
\par The probability that the $i^{th}$ iteration aborts is $\frac{1}{2^{|x|}}$. Conditioned on the $i^{th}$ iteration not aborting, the state $\ket{\Psi_i}$ at the beginning of the $(i+1)^{th}$ iteration is $\sqrt{\varepsilon_{i}}\ket{\phi_1}\ket{1} + \sqrt{\delta_{i}} \ket{\phi_0}\ket{0}$, where:
\begin{itemize}
    \item $\alpha_{i}= \frac{(1 + (2^i - 1)\varepsilon)}{2^i}$ and,
    \item $\delta_i=\frac{\delta_0}{\left( \prod_{j=1}^i \alpha_j \right) \cdot 2^i}$.
\end{itemize}  
\end{lemma}
\begin{proof}
The probability that the $i^{th}$ iteration aborts is $(\beta_i)^{|x|}$ since $\beta_i$ is the probability that the measurement outcome is 1. We calculate $\beta_i$ as follows: 
\begin{eqnarray*}
\beta_i & = & \bra{\Psi_{i-1}} M_1^{\dagger} M_1  \ket{\Psi_{i-1}} \\
& = & \frac{\delta_{i-1}}{2} \leq \frac{1}{2}
\end{eqnarray*}
Thus, we have the probability that the $i^{th}$ iteration aborts is $\frac{1}{2^{|x|}}$. 
\par Suppose the $i^{th}$ iteration does not abort then the state $\ket{\Psi_i}$ is computed as follows: 
 $$\ket{\Psi_i} =  \frac{(I \otimes M_0) \ket{\Psi_{i-1}}}{\sqrt{\alpha_{i}}} = \frac{1}{\sqrt{\alpha_{i}}} \left( \sqrt{\varepsilon_{i-1}} \ket{\phi_1}\ket{1} + \sqrt{\frac{\delta_{i-1}}{2}}\ket{\Psi_{i-1}}\ket{0} \right),$$
           where $\alpha_{i}=\bra{\Psi_{i-1}}M_0^{\dagger} M_0 \ket{\Psi_{i-1}}$.
           \par  We have $\delta_i =\frac{\delta_{i-1}}{2 \alpha_i}$. By substituting in $\delta_{i-1}$, we have that: $\delta_i =  \frac{\delta_0}{\left(\prod_{j=1}^i \alpha_i \right) \cdot 2^i}$. 
    
    
   \noindent Finally, we prove that $\prod_{j=1}^i \alpha_j = \frac{(1 + (2^n - 1)\varepsilon)}{2^n}$.

\begin{eqnarray}
\alpha_{i}= \bra{\Psi_{i}} M_0^{\dagger} M_0 \ket{\Psi_{i}} & = &  \frac{1}{\prod_{j=1}^{i-1} \alpha_j} \left( \frac{1-\varepsilon}{2^{i}} + \varepsilon \right) \\
& = &  \frac{1}{\prod_{j=1}^{i-1} \alpha_j} \cdot \left( \frac{1-\varepsilon}{2^{i}} + \varepsilon \right) \\ 
& = & \frac{1}{\prod_{j=1}^{i-1} \alpha_i} \cdot \left( \frac{1 + (2^{i} - 1) \varepsilon}{2^{i}}\right)
\end{eqnarray}
Now, we have $\prod_{j=1}^{i} \alpha_j = \alpha_{i} \cdot \prod_{j=1}^{i-1} \alpha_j = \frac{1}{\prod_{j=1}^{i-1} \alpha_i} \cdot \left( \frac{1 + (2^{i} - 1) \varepsilon}{2^{i}}\right) \cdot \prod_{j=1}^{i-1} \alpha_i = \left( \frac{1 + (2^{i} - 1) \varepsilon}{2^{i}}\right)$.
\end{proof}

\begin{comment}
\begin{claim}
$p_1 = \frac{n}{2^{|x|}}$.
\end{claim}
\begin{proof}
Fix $i$. We argue in the inner iteration of the algorithm, the probability that the measurement outcome is 
\end{proof}


Denote the state at the end of $i^{th}$ iteration to be $\ket{\Psi_i}$. Without loss of generality, we can denote the state $\ket{\Psi_i}$ as follows: 
$$\ket{\Psi_{i}}= \sqrt{\varepsilon_{i}}\ket{\phi_1}\ket{1} + \sqrt{\delta_{i}}\ket{\phi_0}\ket{0}$$

Consider the following claim.  

\begin{lemma}
For every $i$, suppose at the end of the $i^{th}$ iteration, we get the following state: 
$$\ket{\Psi_{i}}= \sqrt{\varepsilon_{i}}\ket{\phi_1}\ket{1} + \sqrt{\delta_{i}}\ket{\phi_0}\ket{0}$$
Then the 
\end{lemma}
We argue that $\delta_n=  \frac{\delta_0}{\left(\prod_{i=1}^n \alpha_i \right) \cdot 2^n}$, where $\alpha_{i}=\bra{\Psi_{i}}M_0^{\dagger} M_0 \ket{\Psi_{i}}$. Note that ${\delta_0} = {1 - \varepsilon}$. 

\begin{claim}
$\delta_n=\frac{\delta_0}{\left(\prod_{i=1}^n \alpha_i \right) \cdot 2^n}$.
\end{claim}
\begin{proof}
To show this, we first note that $\ket{\Psi_i}$ is computed as follows: 
$$\ket{\Psi_i} =  \frac{(I \otimes M_0) \ket{\Psi_{i-1}}}{\sqrt{\alpha_{i}}} = \frac{1}{\sqrt{\alpha_{i}}} \left( \sqrt{\varepsilon_{i-1}} \ket{\phi_1}\ket{1} + \sqrt{\frac{\delta_{i-1}}{2}}\ket{\Psi_{i-1}}\ket{0} \right)$$
\ \\
We have $\delta_i =\frac{\delta_{i-1}}{2 \alpha_i}$. We prove in the claim below that $\prod_{i=1}^n \alpha_i = \frac{(1 + (2^n - 1)\varepsilon)}{2^n}$. Suppose this is true, then by induction we can argue that $\delta_n =  \frac{\delta_0}{\left(\prod_{i=1}^n \alpha_i \right) \cdot 2^n}$.

\begin{claim}
$\prod_{i=1}^n \alpha_i = \frac{(1 + (2^n - 1)\varepsilon)}{2^n}$. 
\end{claim}
\begin{proof}
We prove by induction. If $\prod_{i=1}^j \alpha_{j} = \frac{(1 + (2^j - 1)\varepsilon)}{2^j}$. Then,
\begin{eqnarray}
\alpha_{j+1}= \bra{\Psi_{j+1}} M_0^{\dagger} M_0 \ket{\Psi_{j+1}} & = &  \frac{1}{\prod_{i=1}^j \alpha_i} \left( \frac{1-\varepsilon}{2^{j+1}} + \varepsilon \right) \\
& = &  \frac{1}{\prod_{i=1}^j \alpha_i} \cdot \left( \frac{1-\varepsilon}{2^{j+1}} + \varepsilon \right) \\ 
& = & \frac{1}{\prod_{i=1}^j \alpha_i} \cdot \left( \frac{1 + (2^{j+1} - 1) \varepsilon}{2^{j+1}}\right)
\end{eqnarray}
Now, we have $\prod_{i=1}^{j+1} \alpha_i = \alpha_{j+1} \cdot \prod_{i=1}^{j} \alpha_i = \frac{1}{\prod_{i=1}^j \alpha_i} \cdot \left( \frac{1 + (2^{j+1} - 1) \varepsilon}{2^{j+1}}\right) \cdot \prod_{i=1}^{j} \alpha_i = \left( \frac{1 + (2^{j+1} - 1) \varepsilon}{2^{j+1}}\right)$. 
\end{proof}

\end{proof}
\end{comment}

\noindent The following lemma will finish the proof of the theorem. 

\begin{lemma}
The probability that the algorithm aborts in any of the $n$ iterations is at most $\frac{n}{2^{|x|}}$. Conditioned on the algorithm not aborting, the final state of the system is the following: 
$$\ket{\Psi_n} = \sqrt{\varepsilon_n} \ket{\phi_1}\ket{1} + \sqrt{\delta_n} \ket{\phi_0}\ket{0},$$
where $\delta_n \leq \frac{2}{3}$. 
\end{lemma}
\begin{proof}
\noindent Thus, we have the following:
\begin{eqnarray*}
\delta_n & = &    \frac{\delta_0}{(\prod_{i=1}^n \alpha_i) \cdot 2^n}\\
& \leq &   \frac{\delta_0}{\left(\frac{2 - \varepsilon}{2^n} \right) \cdot 2^n} \\
& = & \frac{\delta_0}{2 - \varepsilon}\\ & \leq &  \frac{\delta_0}{1.5} \\
& \leq & \frac{2}{3}
\end{eqnarray*}
\end{proof}
\end{proof}
